# Supplementary material for: Test-Time Zero-Shot Temporal Action Localization
Source: arXiv:2404.05426 source file (2024-04-11)
Supplement: Supplementary file 1 [file avg_std.tex]

\begin{table}[ht!]
    \centering
    \begin{tabular}{lccccc|c}
        \toprule
        \textbf{Class} & \multicolumn{6}{c}{\textbf{mAP (\%) $\uparrow$}} \\
                & 0.3 & 0.4 & 0.5 & 0.6 & 0.7 & \textbf{Avg.}  \\ 
        \midrule

        BaseballPitch & 13.2 (3.7) & 9.4 (2.7) & 4.4 (1.5) & 2.5 (0.6) & 1.6 (0.5) \\
        BasketballDunk & 23.5 (3.4) & 13.7 (3.1) & 7.7 (2.4) & 4.1 (1.1) & 1.4 (0.3) \\
        Billiards & 6.9 (3.0) & 4.0 (1.8) & 2.2 (1.2) & 1.2 (0.7) & 0.2 (0.2) \\
        CleanAndJerk & 43.4 (9.6) & 31.8 (9.9) & 22.8 (8.5) & 14.1 (6.0) & 6.8 (2.2) \\
        CliffDiving & 33.4 (6.3) & 23.4 (6.6) & 14.5 (4.3) & 9.1 (2.9) & 4.7 (1.0) \\
        CricketBowling & 7.6 (3.5) & 2.6 (1.1) & 0.9 (0.7) & 0.3 (0.3) & 0.1 (0.1) \\
        CricketShot & 7.1 (0.8) & 3.3 (0.7) & 1.2 (0.3) & 0.5 (0.2) & 0.2 (0.1) \\
        Diving & 23.9 (8.0) & 17.8 (5.6) & 11.7 (3.5) & 6.2 (1.1) & 2.8 (0.2) \\
        FrisbeeCatch & 8.2 (2.0) & 4.0 (1.4) & 1.7 (0.6) & 0.7 (0.5) & 0.4 (0.4) \\
        GolfSwing & 18.1 (2.3) & 10.6 (2.5) & 3.6 (0.9) & 1.3 (0.6) & 0.8 (0.4) \\
        HammerThrow & 34.9 (1.4) & 30.8 (2.3) & 23.3 (1.2) & 15.4 (0.9) & 10.7 (1.6) \\
        HighJump & 30.3 (13.5) & 20.3 (9.7) & 12.2 (6.4) & 5.9 (3.0) & 2.9 (1.6) \\
        JavelinThrow & 29.2 (10.0) & 21.0 (10.6) & 13.8 (11.6) & 8.3 (8.1) & 4.6 (5.5) \\
        LongJump & 51.2 (2.4) & 42.6 (1.9) & 32.5 (1.8) & 21.6 (2.9) & 11.4 (0.9) \\
        PoleVault & 42.0 (3.0) & 33.3 (2.0) & 23.9 (1.7) & 16.6 (1.9) & 7.9 (1.6) \\
        Shotput & 17.1 (5.0) & 12.2 (4.3) & 8.0 (3.0) & 4.8 (2.6) & 2.8 (1.4) \\
        SoccerPenalty & 26.7 (4.7) & 14.0 (2.8) & 6.7 (1.0) & 3.0 (1.1) & 0.8 (0.4) \\
        TennisSwing & 3.8 (1.8) & 2.0 (1.1) & 1.0 (0.5) & 0.5 (0.3) & 0.1 (0.1) \\
        ThrowDiscus & 4.8 (3.2) & 3.5 (2.6) & 2.1 (1.8) & 1.7 (1.9) & 0.7 (0.9) \\
        VolleyballSpiking & 19.6 (1.0) & 14.3 (1.2) & 7.7 (0.9) & 4.1 (1.1) & 2.0 (0.6) \\
        \bottomrule
    \end{tabular}
    \caption{}
    \label{tab:supp_crossdataset}
\end{table}
