# Supplementary material for: Test-Time Zero-Shot Temporal Action Localization
Source: arXiv:2404.05426 source file (2024-04-11)
Supplement: Supplementary file 2 [file thumos_split0.tex]

\begin{table}[h!]
\begin{tabular}{l|ccccc}
\hline                                                                                
 Class        & 0.3 & 0.4 & 0.5 & 0.6 & 0.7 \\                                      
\hline                                                              
 BaseballPitch &    12.9 &     9.5 &     4.6 &     2.5 &     2.2 \\                                                   
 Billiards     &     8.2 &     4.6 &     2.6 &     1.4 &     0.3 \\
 CleanAndJerk  &    46.8 &    35.8 &    24.5 &    16   &     7.8 \\
 GolfSwing     &    20.0 &    11.4 &     3.4 &     1.2 &     0.6 \\
 HammerThrow   &    33.7 &    30.1 &    23.8 &    15.1 &     9.9 \\                                                   
 HighJump      &    40.0 &    29.1 &    18.1 &     8.6 &     4.7 \\                                                   
 PoleVault     &    43.8 &    33.6 &    23.9 &    16.1 &     8.1 \\                                                   
 SoccerPenalty &    29.8 &    15.7 &     6.5 &     2.7 &     0.5 \\                                                   
 TennisSwing   &     4.3 &     2.6 &     1.7 &     0.5 &     0.1 \\                                                   
 ThrowDiscus   &     3.8 &     1.7 &     0.6 &     0.3 &     0.1 \\     
\hline
\end{tabular}
\end{table}
