# Supplementary material for: Test-Time Zero-Shot Temporal Action Localization
Source: arXiv:2404.05426 source file (2024-04-11)
Supplement: Supplementary file 3 [file thumos_split1.tex]

\begin{table}
\begin{tabular}{l|ccccc}
\hline                                                                                
 Class        & 0.3 & 0.4 & 0.5 & 0.6 & 0.7 \\                                      
\hline                                                              
 BaseballPitch     &    17.1 &    12.1 &     6.6 &     2.9 & 1.9      \\
 BasketballDunk    &    24.1 &    14.6 &     8.6 &     4.4 & 1.3      \\
 CricketBowling    &     5.4 &     2.6 &     0.4 &     0.1 & 0.0        \\
 CricketShot       &     6.8 &     3.0 &     1.2 &     0.7 & 0.3      \\
 GolfSwing         &    16.4 &     7.9 &     2.8 &     1.1 & 0.9      \\
 HighJump          &    45.1 &    29.5 &    17.4 &     8.1 & 3.3      \\
 Shotput           &    23.3 &    16.4 &     9.3 &     5.5 & 3.3      \\
 SoccerPenalty     &    28.6 &    15.0 &     6.9 &     1.8 & 0.7      \\
 TennisSwing       &     2.3 &     1.3 &     0.6 &     0.4 & 0.1      \\
 VolleyballSpiking &    19.3 &    14.1 &     7.0 &     3.6 & 2.5      \\
\hline
\end{tabular}
\end{table}
