# Supplementary material for: Test-Time Zero-Shot Temporal Action Localization
Source: arXiv:2404.05426 source file (2024-04-11)
Supplement: Supplementary file 4 [file thumos_split2.tex]

\begin{table}
\begin{tabular}{l|ccccc}
\hline                                                                                
 Class        & 0.3 & 0.4 & 0.5 & 0.6 & 0.7 \\                                      
\hline                                                                          
 BaseballPitch     &     7.9 &     5.9 &     4.3 &     2.9 &     1.1 \\
 CleanAndJerk      &    47.3 &    37.2 &    30.6 &    19.9 &     7.7 \\
 CricketShot       &     6.6 &     2.9 &     0.9 &     0.4 &     0.1 \\                                              
 Diving            &    27.9 &    20.6 &    13.5 &     7.1 &     3.0   \\
 FrisbeeCatch      &     6.2 &     2.5 &     1.2 &     0.3 &     0.1 \\
 GolfSwing         &    18.3 &    10.9 &     4.4 &     1.8 &     1.0   \\
 LongJump          &    48.6 &    40.4 &    30.7 &    18.4 &    10.4 \\
 Shotput           &    14.4 &    10.3 &     6.6 &     3.8 &     1.8 \\
 TennisSwing       &     6.2 &     3.6 &     1.5 &     0.9 &     0.2 \\
 VolleyballSpiking &    20.7 &    15.7 &     9.1 &     5.7 &     2.8 \\                                               
\hline   
\end{tabular}
\end{table}
