# Supplementary material for: Test-Time Zero-Shot Temporal Action Localization
Source: arXiv:2404.05426 source file (2024-04-11)
Supplement: Supplementary file 5 [file thumos_split3.tex]

\begin{table}
\begin{tabular}{l|ccccc}
\hline                                                                                
 Class        & 0.3 & 0.4 & 0.5 & 0.6 & 0.7 \\                                      
\hline                                                              
 BaseballPitch  & 11.6      &     7.6 &     2.5 &  1.5      &  1.0        \\   
 BasketballDunk & 19.6      &     9.7 &     4.9 &  2.8      &  1.2      \\              
 Billiards      &  2.5      &     1.4 &     0.4 &  0.2      &  0.0        \\           
 CleanAndJerk   & 55.3      &    43.9 &    32.4 & 20.5      &  9.7      \\         
 CricketBowling &  4.1      &     1.4 &     0.5 &  0.2      &  0.1      \\          
 CricketShot    &  7.8      &     4.5 &     1.4 &  0.8      &  0.4      \\          
 FrisbeeCatch   &  6.8      &     3.3 &     1.2 &  0.3      &  0.1      \\         
 JavelinThrow   & 37.9      &    32.4 &    26.9 & 17.6      & 11.0        \\         
 Shotput        & 18.0      &    13.5 &     9.4 &  6.6      &  3.4      \\        
 SoccerPenalty  & 28.3      &    13.8 &     7.3 &  4.9      &  1.3      \\  
\hline
\end{tabular}
\end{table}
