# Supplementary material for: Test-Time Zero-Shot Temporal Action Localization
Source: arXiv:2404.05426 source file (2024-04-11)
Supplement: Supplementary file 6 [file thumos_split4.tex]

\begin{table}
\begin{tabular}{l|ccccc}
\hline                                                                                
 Class        & 0.3 & 0.4 & 0.5 & 0.6 & 0.7 \\                                      
\hline                                                              
CliffDiving       &    30.3 &    20.4 &    13.5 &     8.2 &     4.4 \\                                                                  
CricketBowling    &    13.3 &     3.8 &     1.7 &     0.7 &     0.2 \\      
FrisbeeCatch      &     9.5 &     5.0 &     1.9 &     1.2 &     0.9 \\              
HammerThrow       &    36.4 &    33.4 &    24.2 &    16.5 &    12.6 \\               
HighJump          &    33.9 &    22.6 &    14.9 &     7.4 &     4.1 \\              
PoleVault         &    41.5 &    33.3 &    23.4 &    15.5 &     6.3 \\             
SoccerPenalty     &    26.3 &    14.7 &     7.6 &     3.7 &     1.4 \\             
TennisSwing       &     2.4 &     0.8 &     0.4 &     0.2 &     0.0 \\               
ThrowDiscus       &     1.9 &     1.3 &     0.9 &     0.1 &     0.0 \\              
VolleyballSpiking &    19.7 &    15.5 &     8.4 &     4.7 &     2.1 \\ 
\hline
\end{tabular}
\end{table}
