# Supplementary material for: Test-Time Zero-Shot Temporal Action Localization
Source: arXiv:2404.05426 source file (2024-04-11)
Supplement: Supplementary file 7 [file thumos_split5.tex]

\begin{table}
\begin{tabular}{l|ccccc}
\hline                                                                                
 Class        & 0.3 & 0.4 & 0.5 & 0.6 & 0.7 \\                                      
\hline       
BasketballDunk &    22.5 &    13.3 &     6.8 &     3.8 &     1.1 \\    
 Billiards      &     9.3 &     4.8 &     2.7 &     1.4 &     0.1 \\                
 CliffDiving    &    40.6 &    30.9 &    19.2 &    12.4 &     5.9 \\                 
 CricketBowling &     6.6 &     2.6 &     0.8 &     0.1 &     0.1 \\                 
 CricketShot    &     8.3 &     3.6 &     1.5 &     0.7 &     0.2 \\                
 GolfSwing      &    17.3 &    11.4 &     4.4 &     1.0  &     0.3 \\              
 PoleVault      &    41.6 &    32.7 &    22.7 &    15.4 &     7.5 \\               
 Shotput        &    22.4 &    17.7 &    12.5 &     8.7 &     5.1 \\                
 TennisSwing    &     4.7 &     2.1 &     1.1 &     0.6 &     0.1 \\                
 ThrowDiscus    &     4.3 &     3.1 &     1.8 &     1.3 &     0.4 \\ 
\hline
\end{tabular}
\end{table}
