# Supplementary material for: Test-Time Zero-Shot Temporal Action Localization
Source: arXiv:2404.05426 source file (2024-04-11)
Supplement: Supplementary file 8 [file thumos_split6.tex]

\begin{table}
\begin{tabular}{l|ccccc}
\hline                                                                                
 Class        & 0.3 & 0.4 & 0.5 & 0.6 & 0.7 \\                                      
\hline                                                     
CleanAndJerk   & 26.9      & 14.9      &     9.2 &     5.6 &     3.8 \\
 CliffDiving    & 29.2      & 18.8      &    10.8 &     6.8 &     3.9 \\
 CricketBowling &  5.7      &  1.5      &     0.4 &     0.2 &     0.1 \\
 CricketShot    &  6.4      &  3.5      &     1.4 &     0.5 &     0.2 \\
 HighJump       & 18.0      & 10.2      &     5.1 &     2.8 &     1.5 \\
 JavelinThrow   & 18.3      & 11.4      &     5.0 &     2.8 &     1.0 \\
 LongJump       & 53.3      & 43.7      &    32.5 &    22.2 &    11.7 \\
 PoleVault      & 39.1      & 32.4      &    24.4 &    16.4 &     7.1 \\
 SoccerPenalty  & 18.3      &  9.9      &     4.6 &     2.1 &     0.5 \\
 TennisSwing    &  1.1      &  0.5      &     0.3 &     0.0 &     0.0 \\         

\hline
\end{tabular}
\end{table}
