# Supplementary material for: Test-Time Zero-Shot Temporal Action Localization
Source: arXiv:2404.05426 source file (2024-04-11)
Supplement: Supplementary file 9 [file thumos_split7.tex]

\begin{table}
\begin{tabular}{l|ccccc}
\hline                                                                                
 Class        & 0.3 & 0.4 & 0.5 & 0.6 & 0.7 \\                                      
\hline                                                              
BaseballPitch     & 16.3      &    11.9 &     4.0 &     2.6 &     1.8 \\
CleanAndJerk      & 39.1      &    28.3 &    18.4 &     8.6 &     4.6 \\
CricketShot       &  6.2      &     2.3 &     1.1 &     0.4 &     0.1 \\
Diving            & 14.7      &    11.3 &     7.7 &     4.9 &     2.6 \\
HighJump          & 14.5      &    10.1 &     5.5 &     2.6 &     0.9 \\
PoleVault         & 39.1      &    31.0 &    21.9 &    15.8 &     7.4 \\
Shotput           & 12.8      &     8.2 &     5.1 &     1.8 &     1.0 \\
TennisSwing       &  4.1      &     2.3 &     1.3 &     0.6 &     0.2 \\
ThrowDiscus       &  3.9      &     3.4 &     2.0 &     1.8 &     0.9 \\
VolleyballSpiking & 20.4      &    12.7 &     7.8 &     4.6 &     1.5 \\
\hline
\end{tabular}
\end{table}
