# Supplementary material for: Test-Time Zero-Shot Temporal Action Localization
Source: arXiv:2404.05426 source file (2024-04-11)
Supplement: Supplementary file 10 [file thumos_split8.tex]

\begin{table}
\begin{tabular}{l|ccccc}
\hline                                                                                
 Class        & 0.3 & 0.4 & 0.5 & 0.6 & 0.7 \\                                      
\hline                                                              
CricketBowling    &    10.5 &     4.0  &  1.8      &     0.7 &     0.3 \\                                  
 FrisbeeCatch      &    10.3 &     5.4 &  2.4      &     1.1 &     0.5 \\                                   
 GolfSwing         &    21.4 &    14.4 &  4.4      &     2.1 &     1.4 \\                                   
 HammerThrow       &    34.7 &    29.0 & 21.9      &    14.7 &     9.7 \\                                   
 LongJump          &    51.7 &    43.7 & 34.2      &    24.1 &    12.2 \\                                    
 PoleVault         &    47.0 &    36.9 & 26.9      &    20.5 &    10.9 \\                                   
 Shotput           &    11.6 &     7.3 &  4.9      &     2.6 &     2.4 \\                                  
 SoccerPenalty     &    23.2 &    11.1 &  6.4      &     2.1 &     0.6 \\                                 
 TennisSwing       &     5.6 &     3.0 &  1.4      &     0.7 &     0.3 \\
 VolleyballSpiking &    17.8 &    13.3 &  7.3      &     3.3 &     1.8 \\
\hline
\end{tabular}
\end{table}
