# Supplementary material for: Test-Time Zero-Shot Temporal Action Localization
Source: arXiv:2404.05426 source file (2024-04-11)
Supplement: Supplementary file 11 [file thumos_split9.tex]

\begin{table}
\begin{tabular}{l|ccccc}
\hline                                                                                
 Class        & 0.3 & 0.4 & 0.5 & 0.6 & 0.7 \\                                      
\hline                                                        
BasketballDunk    &    27.7 &    17.2 &    10.5 &     5.5 &     1.8 \\   
 Billiards         &     7.5 &     5.2 &     2.9 &     1.7 &     0.3 \\                  
 CleanAndJerk      &    45.2 &    31.0 &    21.7 &    14.0 &     6.9 \\                
 CricketShot       &     7.4 &     3.4 &     0.8 &     0.3 &     0.1 \\                
 Diving            &    29.0 &    21.5 &    13.9 &     6.5 &     2.8 \\               
 GolfSwing         &    15.1 &     7.9 &     2.3 &     0.5 &     0.4 \\                  
 JavelinThrow      &    31.3 &    19.2 &     9.4 &     4.6 &     1.9 \\               
 SoccerPenalty     &    32.4 &    18.1 &     7.6 &     3.7 &     0.7 \\              
 ThrowDiscus       &    10.3 &     7.8 &     5.2 &     4.9 &     2.2 \\                 
 VolleyballSpiking &    19.6 &    14.3 &     6.6 &     2.7 &     1.1 \\
\hline
\end{tabular}
\end{table}
